# Supplementary material for: Influential Observations in Bayesian Regression Tree Models
Source: arXiv:2203.14102 source file (2023-05-17)
Supplement: Supplementary file 1 [file supplement.pdf]

# Supplement

## Proof of Equation (2)

Recall for linear models the Cook's distance metric for observation  $i$  can be expressed as (Weisberg, 2013):

$$D_i = \frac{\sum_{j=1}^n (\hat{y}_j - \hat{y}_{j(i)})^2}{ds^2} = \frac{1}{p} \left( \frac{e_i}{s} \right)^2 \frac{h_{ii}}{1 - h_{ii}}.$$

For our single-tree model, we have  $p = B$  and we replace  $s^2$  with a posterior sample of the variance, say  $\sigma$ . Then, we need only simplify the expression involving  $h_{ii}$ . Let  $F_j$  represent a vector of indicators where

$$F_{ji} = \begin{cases} 1 & \text{if } x_i \in \text{terminal node } j \\ 0 & \text{otherwise} \end{cases}.$$

By construction, note that  $F_j^T F_k = 0$  for all column vectors  $F_j, F_k$  such that  $k \neq j$ , and  $F_j^T F_j = n_j$ , the number of observations mapping to terminal node  $j$ . Now suppose observation  $x_i$  maps to terminal node  $j$ , resulting in  $f_i$  being a vector of zeros except in position  $j$  (which is a 1). Then,

$$\begin{aligned} h_{ii} &= f_i^T (F^T F)^{-1} f_i \\ &= f_i^T \begin{pmatrix} F_1^T F_1 & 0 & \cdots & 0 \\ 0 & F_2^T F_2 & \cdots & \vdots \\ \vdots & \vdots & \ddots & \vdots \\ 0 & \cdots & \cdots & F_B^T F_B \end{pmatrix} f_i \\ &= f_i^T \text{diag}(n_1^{-1}, \dots, n_B^{-1}) f_i \\ &= n_j^{-1}. \end{aligned}$$

Substituting,  $\frac{h_{ii}}{(1-h_{ii})^2} = \frac{n_j}{(n_j-1)^2}$ , and the resulting form of Cook's Distance in Equation (2) results.

## Proof of Proposition 0.

First, we interpret the ratio as  $\frac{\pi(\mathbf{Y}_{-i})}{\pi(\mathbf{Y})} = [\pi(y_i|\mathbf{Y}_{-i})]^{-1}$ . Now,

$$\begin{aligned}\pi(y_i|\mathbf{Y}_{-i}) &= \int_{\Theta} \pi(y_i|\mathbf{Y}_{-i}, \Theta)\pi(\Theta|\mathbf{Y}_{-i})d\Theta \\ &= \int_{\Theta} \pi(y_i|\mathbf{Y}_{-i}, \Theta)\frac{\pi(\Theta|\mathbf{Y}_{-i})}{\pi(\Theta|\mathbf{Y})}\pi(\Theta|\mathbf{Y})d\Theta \\ &\equiv E_{\Theta} [g_i(\Theta)w_i(\Theta)], \quad \Theta \sim \pi(\Theta|\mathbf{Y}),\end{aligned}$$

where  $g_i(\Theta) = \pi(y_i|\mathbf{Y}_{-i}, \Theta) = f(y_i|\Theta)$  since the data are independent conditional on  $\Theta$ , and  $w_i(\Theta) \propto \frac{f(\mathbf{Y}_{-i}|\Theta)}{f(\mathbf{Y}|\Theta)} = [f(y_i|\Theta)]^{-1}$ . Then by the self-normalized importance sampling theorem (e.g. Owen, 2013, Ch.9), we know that the estimator

$$\frac{\sum_{k=1}^N w_i^{(k)} g_i(\Theta^{(k)})}{\sum_{i=1}^N w_i^{(k)}} \rightarrow E_{\Theta} [g_i(\Theta)w_i(\Theta)]$$

as  $N \rightarrow \infty$  by the strong law of large numbers, where  $w_i^{(k)} = w_i(\Theta^{(k)})$ . Therefore, by the continuous mapping theorem, it follows that

$$\log \left( \left[ \frac{\sum_{k=1}^N w_i^{(k)} g_i(\Theta^{(k)})}{\sum_{i=1}^N w_i^{(k)}} \right]^{-1} \right) = \log \left( \frac{1}{N} \sum_{k=1}^N [f(y_i|\Theta^{(k)})]^{-1} \right) \rightarrow \log \left( \frac{\pi(\mathbf{Y}_{-i})}{\pi(\mathbf{Y})} \right).$$

## Proof of Proposition 1.

Suppose  $y_i$  lives in terminal node  $\eta_j$  with mean parameter  $\mu_j$ . Let  $P_j$  represent the path from the terminal node  $j$  back to the tree root, and let  $\tilde{\Theta} = \Theta \setminus \mu_j, P_j, \sigma^2$  represent all other parameters making up the tree. The posterior can then be factored (up to proportionality) as

$$\begin{aligned}\pi(\Theta|\mathbf{Y}) &\propto f(\mathbf{Y}_{(j)}|\mu_j, \eta_j, P_j, \sigma^2)\pi(\eta_j \text{terminal})\pi(\mu_j)\pi(P_j)\pi(\sigma^2)f(\mathbf{Y}_{-(j)}|\tilde{\Theta}, P_j, \sigma^2)\pi(\tilde{\Theta}) \\ &\propto f(\mathbf{Y}_{(j)}|\mu_j, \eta_j, P_j, \sigma^2)\pi(\eta_j \text{terminal})\pi(\mu_j)\pi(P_j)\pi(\sigma^2)\pi(\tilde{\Theta}|\mathbf{Y}_{-(j)}, P_j, \sigma^2)\end{aligned}$$

Integrating, we get

$$\begin{aligned}\int_{\tilde{\Theta}} \pi(\Theta|\mathbf{Y}) &\propto f(\mathbf{Y}_{(j)}|\mu_j, \eta_j, P_j, \sigma^2)\pi(\eta_j \text{terminal})\pi(\mu_j)\pi(P_j)\pi(\sigma^2) \int_{\tilde{\Theta}} \pi(\tilde{\Theta}|\mathbf{Y}_{-(j)}, P_j, \sigma^2)d\tilde{\Theta} \\ &\propto f(\mathbf{Y}_{(j)}|\mu_j, \eta_j, P_j, \sigma^2)\pi(\eta_j \text{terminal})\pi(\mu_j)\pi(P_j)\pi(\sigma^2) \\ &\propto \pi(\mu_j, \eta_j, P_j, \sigma^2|\mathbf{Y}_{(j)})\end{aligned}$$

So we can choose the importance distribution to be  $\pi(\mu_j, \eta_j, P_j, \sigma^2 | \mathbf{Y}_{(j)})$  since posterior samples from the marginal are readily available by simply dropping the unneeded dimensions of  $\Theta$ , so the weights become

$$w_{(i)}^{(k)} = \frac{\pi(\mu_j, \eta_j, P_j, \sigma^2 | \mathbf{Y}_{(j) \setminus i})}{\pi(\mu_j, \eta_j, P_j, \sigma^2 | \mathbf{Y}_{(j)})} \\ \propto \frac{\prod_{l \neq i} f(y_{(j),l} | \mu_j, \eta_j, P_j, \sigma^2) \pi(\mu_j) \pi(\eta_j) \pi(P_j) \pi(\sigma^2) \mathbb{I}(|\eta_j| - 1 \geq n_0)}{\prod_l f(y_{(j),l} | \mu_j, \eta_j, P_j, \sigma^2) \pi(\mu_j) \pi(\eta_j) \pi(P_j) \pi(\sigma^2) \mathbb{I}(|\eta_j| \geq n_0)}$$

and since  $\mathbb{I}(|\eta_j| \geq n_0)$  by definition, we arrive at

$$w_{(i)}^{(k)} \propto \begin{cases} \frac{1}{f(y_i | \mu_j, \eta_j, P_j, \sigma^2)}, & \text{if } |\eta_j| - 1 \geq n_0 \\ 0, & \text{otherwise.} \end{cases}$$

Similarly, suppose we are interested in predictions at terminal node  $\eta_l$  with mean parameter  $\mu_l$  and where  $y_i$  does not live in  $\eta_l$ . Choosing  $\pi(\mu_l, \eta_l, P_l, \sigma^2 | \mathbf{Y}_{(l)})$  to be the importance distribution, we have

$$w_{(i)}^{(k)} = \frac{\pi(\mu_l, \eta_l, P_l, \sigma^2 | \mathbf{Y}_{(l) \setminus i})}{\pi(\mu_l, \eta_l, P_l, \sigma^2 | \mathbf{Y}_{(l)})} \\ = 1,$$

since  $y_i$  does not appear in  $\eta_l$  and therefore does not affect the numerator.

## Proof of Proposition 2

Suppose now we have a BART model involving  $m$  trees. Suppose  $y_i$  lives in terminal nodes  $\eta_{j_1}, \dots, \eta_{j_m}$ . Suppose we want to perform a (weighted) prediction at input setting  $x$ . This prediction input could map exactly to each  $\eta_{j_l}, l = 1, \dots, m$  or only a single  $\eta_{j_l}$  for some  $l \in \{1, \dots, m\}$ , or indeed any subset of terminals between these extremes. We will want to weight if for inputs that map to at least one of these nodes, which means  $m - 1$  nodes will not be in the set  $\eta_{j_1}, \dots, \eta_{j_m}$ . Let  $\boldsymbol{\eta}_a$  represent these nodes and  $\boldsymbol{\eta}_b$  represent the remaining set of nodes that are not involved in predictions at  $x$ . Let  $\boldsymbol{\mu}_a, \mathbf{P}_a$  be the respective mean parameters and paths in the  $m$  trees. Let  $\tilde{\Theta} = \Theta \setminus \boldsymbol{\eta}_a, \boldsymbol{\mu}_a, \mathbf{P}_a, \sigma^2$ . Finally, let  $\mathbf{Y}_a$  and  $\mathbf{Y}_b$  be the respective portions of the dataset. Then,

$$\pi(\Theta | \mathbf{Y}) \propto f(\mathbf{Y}_a | \boldsymbol{\mu}_a, \boldsymbol{\eta}_a, \mathbf{P}_a, \sigma^2) \pi(\boldsymbol{\mu}_a, \boldsymbol{\eta}_a, \mathbf{P}_a) \pi(\sigma^2) f(\mathbf{Y}_b | \tilde{\Theta}, \boldsymbol{\mu}_a, \boldsymbol{\eta}_a, \mathbf{P}_a, \sigma^2) \pi(\tilde{\Theta}) \\ \propto f(\mathbf{Y}_a | \boldsymbol{\mu}_a, \boldsymbol{\eta}_a, \mathbf{P}_a, \sigma^2) \pi(\boldsymbol{\mu}_a, \boldsymbol{\eta}_a, \mathbf{P}_a) \pi(\sigma^2) \pi(\tilde{\Theta} | \mathbf{Y}_b, \boldsymbol{\mu}_a, \boldsymbol{\eta}_a, \mathbf{P}_a, \sigma^2)$$

Integrating, we have

$$\int_{\tilde{\Theta}} \pi(\Theta|\mathbf{Y}) \propto \pi(\boldsymbol{\mu}_a, \boldsymbol{\eta}_a, \mathbf{P}_a, \sigma^2 | \mathbf{Y}_a).$$

The weights for predicting at  $x$  then become

$$w_{(i)}^{(k)}(x) \propto \frac{1}{f(y_i | \boldsymbol{\mu}_a, \boldsymbol{\eta}_a, \mathbf{P}_a, \sigma^2)} \prod_{l: x \in \eta_{jl}} \mathcal{G}(|\eta_j| - 1 \geq n_0).$$

Similarly, if we are interesting in predicting at  $x$  such that  $x$  does not involve any of the  $\eta_{jl}, l = 1, \dots, m$ , then as in Proposition 1 the weight will be 1.

### Proof of Proposition 3

Let  $\mathcal{S}$  be our super-tree representation of the original BART trees  $T_1, \dots, T_m$ . Suppose  $y_i$  lives in terminal node  $\eta_j^{\mathcal{S}}$  with mean parameter  $\mu_j^{\mathcal{S}}$  and let  $P_j^{\mathcal{S}}$  represent the path from terminal node  $j$  back to the super-tree root. Let  $\tilde{\Theta}^{\mathcal{S}} = \Theta^{\mathcal{S}} \setminus \mu_j^{\mathcal{S}}, P_j^{\mathcal{S}}, \sigma^2$  represent all other parameters making up the super-tree. Then,

$$\begin{aligned} \pi(\Theta^{\mathcal{S}} | \mathbf{Y}) &\propto f(\mathbf{Y}_{(j)} | \mu_j^{\mathcal{S}}, \eta_j^{\mathcal{S}}, P_j^{\mathcal{S}}, \sigma^2) \pi(\eta_j^{\mathcal{S}} \text{ terminal}) \pi(\mu_j^{\mathcal{S}}) \pi(P_j^{\mathcal{S}}) \pi(\sigma^2) f(\mathbf{Y}_{-(j)} | \tilde{\Theta}^{\mathcal{S}}, P_j^{\mathcal{S}}, \sigma^2) \pi(\tilde{\Theta}^{\mathcal{S}}) \\ &\propto f(\mathbf{Y}_{(j)} | \mu_j^{\mathcal{S}}, \eta_j^{\mathcal{S}}, P_j^{\mathcal{S}}, \sigma^2) \pi(\eta_j^{\mathcal{S}} \text{ terminal}) \pi(\mu_j^{\mathcal{S}}) \pi(P_j^{\mathcal{S}}) \pi(\sigma^2) \pi(\tilde{\Theta}^{\mathcal{S}} | \mathbf{Y}_{-(j)}, P_j^{\mathcal{S}}, \sigma^2). \end{aligned}$$

Integrating, we get

$$\int_{\tilde{\Theta}^{\mathcal{S}}} \pi(\Theta^{\mathcal{S}} | \mathbf{Y}) \propto \pi(\mu_j^{\mathcal{S}}, \eta_j^{\mathcal{S}}, P_j^{\mathcal{S}}, \sigma^2 | \mathbf{Y}_{(j)})$$

and the weights for predicting at  $x \in \eta_j^{\mathcal{S}}$  become

$$w_{(i)}^{(k)}(x) \propto \frac{1}{f(y_i | \mu_j^{\mathcal{S}}, \eta_j^{\mathcal{S}}, P_j^{\mathcal{S}}, \sigma^2)} \prod_{l: x \in \eta_{kl}} \mathcal{G}(|\eta_{kl}| - 1 \geq n_0).$$

Note here that  $\eta_j^{\mathcal{S}} = \cap_{l=1}^m \eta_{kl}$  for nodes  $\eta_{kl}$  in the original BART ensemble to which  $x$  maps.

Finally, as in Proposition 1, predicting at an  $x$  that does not involve  $\eta_j^{\mathcal{S}}$  has corresponding weight 1.
