# Supplementary material for: Influential Observations in Bayesian Regression Tree Models
Source: arXiv:2203.14102 source file (2023-05-17)
Supplement: Supplementary file 2 [file supp.tex]

\subsection*{Proof of Equation (2)}
Recall for linear models the Cook's distance metric for observation $i$ can be expressed as \citep{weisberg2013applied}:
$$D_i=\frac{\sum_{j=1}^n\left(\hat{y}_j-\hat{y}_{j(i)}\right)^2}{ds^2}=\frac{1}{p}\left(\frac{e_i}{s}\right)^2
\frac{h_{ii}}{1-h_{ii}}.
$$
For our single-tree model, we have $p=B$ and we replace $s^2$ with a posterior sample of the variance, say $\sigma$.  Then, we need only simplify the expression involving $h_{ii}.$  Let $F_j$ represent a vector of indicators where $$F_{ji}=\begin{cases}
1 & \text{ if } x_i \in \text{ terminal node } j\\
0 & \text{ otherwise}
\end{cases}
.$$
By construction, note that $F^T_jF_k=0$ for all column vectors $F_j,F_k$ such that $k\neq j$, and $F_j^TF_j=n_j$, the number of observations mapping to terminal node $j.$  Now suppose observation $x_i$ maps to terminal node $j$, resulting in $f_i$ being a vector of zeros except in position $j$ (which is a 1).  Then,
\begin{align*}
h_{ii} &= f_i^T\left(F^TF\right)^{-1}f_i\\
&= f_i^T\left(\begin{array}{cccc}
F_1^TF_1 & 0 & \cdots & 0 \\
0 & F_2^TF_2 & \cdots & \vdots \\
\vdots   & \vdots   & \ddots & \vdots \\
0   & \cdots   & \cdots & F_B^TF_B\\
\end{array}\right)f_i \\
&= f_i^T \text{diag}\left(n_1^{-1},\ldots,n_B^{-1})\right)f_i \\
&= n_j^{-1}.
\end{align*}
Substituting, $\frac{h_{ii}}{(1-h_{ii})^2}=\frac{n_j}{(n_j-1)^2},$ and the resulting form of Cook's Distance in Equation (2) results.



\subsection*{Proof of Proposition 0.}
First, we interpret the ratio as $\frac{\pi({\bf Y}_{-i})}{\pi({\bf Y})}=[\pi(y_i\vert {\bf Y}_{-i})]^{-1}.$  Now,
\begin{align*}
\pi(y_i\vert {\bf Y}_{-i}) &= \int_{\Theta}\pi(y_i\vert{\bf Y}_{-i},\Theta)\pi(\Theta\vert{\bf Y}_{-i})d\Theta\\
&= \int_{\Theta}\pi(y_i\vert{\bf Y}_{-i},\Theta)\frac{\pi(\Theta\vert{\bf Y}_{-i})}{\pi(\Theta\vert{\bf Y})}\pi(\Theta\vert{\bf Y})d\Theta\\
&\equiv E_\Theta\left[g_i(\Theta)w_i(\Theta)\right],\ \ \Theta\sim\pi(\Theta\vert{\bf Y}),
\end{align*}
where $g_i(\Theta)=\pi(y_i\vert{\bf Y}_{-i},\Theta)=f(y_i\vert\Theta)$ since the data are independent conditional on $\Theta,$ and $w_i(\Theta)\propto \frac{f({\bf Y}_{-i}\vert\Theta)}{f({\bf Y}\vert\Theta)}=\left[f(y_i\vert\Theta)\right]^{-1}.$
Then by the self-normalized importance sampling theorem \citep[e.g.][Ch.9]{mcbook}, we know that the estimator 
$$\frac{\sum_{k=1}^N w_i^{(k)}g_i(\Theta^{(k)})}{\sum_{i=1}^Nw_i^{(k)}}\rightarrow E_\Theta\left[g_i(\Theta)w_i(\Theta)\right]$$ 
as $N\rightarrow\infty$ by the strong law of large numbers, where $w_i^{(k)}=w_i(\Theta^{(k)}).$  Therefore, by the continuous mapping theorem, it follows that
$$\log\left(\left[\frac{\sum_{k=1}^N w_i^{(k)}g_i(\Theta^{(k)})}{\sum_{i=1}^Nw_i^{(k)}}\right]^{-1}\right)=\log\left(\frac{1}{N}\sum_{k=1}^N[f(y_i\vert\Theta^{(k)})]^{-1}\right)\rightarrow \log\left(\frac{\pi({\bf Y}_{-i})}{\pi({\bf Y})}\right).$$


\subsection*{Proof of Proposition 1.}

Suppose $y_i$ lives in terminal node $\eta_j$ with mean parameter $\mu_j.$    
Let $P_j$ represent the path from the terminal node $j$ back to the tree root, and let $\tilde{\Theta}=\Theta\setminus\mu_j,P_j,\sigma^2$ represent all other parameters making up the tree.  The posterior can then be factored (up to proportionality) as
\begin{align*}
\label{eqn:singletreepost}
\pi(\Theta\vert{\bf Y}) &\propto f({\bf Y}_{(j)}\vert \mu_j,\eta_j,P_j,\sigma^2)\pi(\eta_j \text{terminal})\pi(\mu_j)\pi(P_j)\pi(\sigma^2)f({\bf Y}_{-(j)}\vert\tilde{\Theta},P_j,\sigma^2)\pi(\tilde{\Theta})\\
&\propto f({\bf Y}_{(j)}\vert \mu_j,\eta_j,P_j,\sigma^2)\pi(\eta_j  \text{terminal})\pi(\mu_j)\pi(P_j)\pi(\sigma^2)\pi(\tilde{\Theta}\vert {\bf Y}_{-(j)},P_j,\sigma^2)
%\pi(\theta\vert{\bf Y}) &\propto \pi(\mu_j\vert {\bf Y}_{(j)},P_j,\sigma^2)\pi(\tilde{\theta},P_j,\sigma^2\vert{\bf Y})\\
%&\propto \pi(\mu_j\vert{\bf Y},P_j,\sigma^2)\pi(\tilde{\theta}\vert {\bf Y},P_j\sigma^2)\pi(P_j,\sigma^2\vert{\bf y})
%%\pi(\theta\vert{\bf Y}) &\propto \prod_{i=1}^n\pi(y_i\vert\theta)\pi(\theta)\\ \nonumber
%%&=\prod_{i\in\eta_j}\pi(y_i\vert\mu_j)\pi(\mu_j)\prod_{\eta_k\setminus\eta_j}\pi(y_k\vert\mu_k)\pi(\mu_k)\prod_{l:\eta_l\in P_j\setminus\mu_j\setminus B_{j\setminus\mu_j}}\pi(v_l)\pi(c_l\vert v_l)\pi(\eta_l \text{ is non-terminal})\\ \nonumber
%%&\ \times \prod_{l:\eta_l\in P_j\setminus\mu_j\setminus B_{j\setminus\mu_j}}\eta_l\in\bar{P}_{j\setminus\mu_j}\pi(v_l)\pi(c_l\vert v_l)\pi(v_l \text{ is non-terminal})\\ \nonumber
%%&\ \times \prod_{l:\eta_l\in B{j\setminus\mu_j}}\pi(\eta_l \text{ is terminal})\pi(\eta_j\text{ is terminal}).\nonumber
\end{align*}
Integrating, we get
\begin{align*}
%\int_{\tilde{\theta}}\pi(\theta\vert{\bf Y}) &= \int_{\tilde{\theta}} \pi(\mu_j\vert {\bf Y}_{(j)},P_j,\sigma^2)\pi(\tilde{\theta}\vert{\bf Y},P_j,\sigma^2)\pi(P_j,\sigma^2\vert{\bf Y})\\
\int_{\tilde{\Theta}}\pi(\Theta\vert{\bf Y}) &\propto f({\bf Y}_{(j)}\vert\mu_j,\eta_j,P_j,\sigma^2)\pi(\eta_j \text{terminal})\pi(\mu_j)\pi(P_j)\pi(\sigma^2)\int_{\tilde{\Theta}} \pi(\tilde{\Theta}\vert{\bf Y}_{-(j)},P_j,\sigma^2)d\tilde{\Theta}\\
&\propto f({\bf Y}_{(j)}\vert\mu_j,\eta_j,P_j,\sigma^2)\pi(\eta_j \text{terminal})\pi(\mu_j)\pi(P_j)\pi(\sigma^2)\\
&\propto\pi(\mu_j,\eta_j,P_j,\sigma^2\vert{\bf Y}_{(j)})
\end{align*}
So we can choose the importance distribution to be $\pi(\mu_j,\eta_j,P_j,\sigma^2\vert{\bf Y}_{(j)})$ since posterior samples from the marginal are readily available by simply dropping the unneeded dimensions of $\Theta$, so the weights become
\begin{align*}
w_{(i)}^{(k)} &= \frac{\pi(\mu_j,\eta_j,P_j,\sigma^2\vert{\bf Y}_{(j)\setminus  i})}{\pi(\mu_j,\eta_j,P_j,\sigma^2\vert{\bf Y}_{(j)})}\\
&\propto \frac{\prod_{l\neq i}f(y_{(j),l}\vert\mu_j,\eta_j,P_j,\sigma^2)\pi(\mu_j)\pi(\eta_j)\pi(P_j)\pi(\sigma^2)\mathbb{I}(\vert\eta_j\vert-1\geq \minbot)}{\prod_{l}f(y_{(j),l}\vert\mu_j,\eta_j,P_j,\sigma^2)\pi(\mu_j)\pi(\eta_j)\pi(P_j)\pi(\sigma^2)\mathbb{I}(\vert\eta_j\vert\geq \minbot)} 
\end{align*}
and since $\mathbb{I}(\vert\eta_j\vert\geq \minbot)$ by definition, we arrive at
\begin{align*}
w_{(i)}^{(k)} &\propto \begin{cases} \frac{1}{f(y_i\vert\mu_j,\eta_j,P_j,\sigma^2)}, \text{ if } \vert\eta_j\vert-1\geq \minbot\\
0, \text{ otherwise.}
\end{cases}
\end{align*}

Similarly, suppose we are interested in predictions at terminal node $\eta_l$ with mean parameter $\mu_l$ and where $y_i$ does not live in $\eta_l.$  Choosing $\pi(\mu_l,\eta_l,P_l,\sigma^2\vert{\bf Y}_{(l)})$ to be the importance distribution, we have
\begin{align*}
w_{(i)}^{(k)} &= \frac{\pi(\mu_l,\eta_l,P_l,\sigma^2\vert{\bf Y}_{(l)\setminus i})}{\pi(\mu_l,\eta_l,P_l,\sigma^2\vert{\bf Y}_{(l)})}\\
%&\propto \frac{\prod_{m}f(y_m\vert\mu_l,P_l,\sigma^2)\pi(\mu_l)\pi(P_l)\pi(\sigma^2)\mathbb{I}(\vert\eta_l\vert\geq \minbot)}{\prod_{m}f(y_m\vert\mu_j,P_l,\sigma^2)\pi(\mu_l)\pi(P_l)\pi(\sigma^2)\mathbb{I}(\vert\eta_l\vert\geq \minbot)} \\
&= 1,
\end{align*}
since $y_i$ does not appear in $\eta_l$ and therefore does not affect the numerator.


%Recall that since we assume the functional of interest is merely $g(\theta):=g(\mu_j)$ (i.e. the case of prediction), then given the above factorization most of the terms not involving $\mu_j$ cancel in the ratio for calculating the weight.  Writing $\pi(y_i\vert\mu_j)=\text{N}(y_i;\mu_j,\sigma^2)\text{I}_{\vert\eta_j\vert\geq\minbot},$ where $N(\cdot)$ denotes the \alphaian p.d.f. and $I$ represents the indicator function, we then have
%
%\begin{align*}
%\frac{\pi(\theta\vert{\bf Y}_{-i})}{\pi(\theta\vert{\bf Y})} &\propto
%\frac{\prod_{k\in\eta_j,k\neq i}\text{N}(y_k\vert\mu_j,\sigma^2)\text{I}[\vert\eta_j\vert-1\geq\minbot]\prod_{l\in s(\eta_j)}\text{I}[\vert \eta_l\vert\geq \minbot]}{\prod_{k\in\eta_j}\text{N}(y_k\vert\mu_j,\sigma^2)\text{I}[\vert\eta_j\vert\geq\minbot]\prod_{l\in s(\eta_j)}\text{I}[\vert \eta_l\vert\geq \minbot]},\\
%\end{align*}
%
%where $s(\eta_j)$ denotes terminal node siblings to terminal node $\eta_j$ (i.e. terminal nodes on the other branch of the parent node of $\eta_j$).
%Here, the indicator functions in the denominator must evaluate to 1 for the tree to have been arrived at by the MCMC algorithm (it is guaranteed to be valid), and similarly the terms $\text{I}[\vert \eta_l\vert\geq \minbot]$ in the numerator must evaluate to 1 in the case-deleted likelihood as the deletion only affects node $\eta_j$, not $\eta_j$'s sibling terminal node(s).  Crucially, note that most of the terms in the full posterior equation (\ref{eqn:singletreepost}) cancel out, so upon simplifying we arrive at
%
%\begin{align*}
%\frac{\pi(\theta\vert{\bf Y}_{-i})}{\pi(\theta\vert{\bf Y})} &\propto 
%\begin{cases}
%\frac{1}{\text{N}(y_i\vert \mu_j,\sigma^2)} \textbf{ if } \vert\eta_j\vert-1\geq \minbot\\
%0 \textbf{ otherwise},
%\end{cases}
%\end{align*}
%
%as required.  Note that this result still holds in the case that $\minbot=0.$  In words, this result says that when we hold-out $y_i$, the weights for reweighting predictions involving $mu_j$ by the inverse density in $y_i$ if the node would have been valid with the case deleted, otherwise the prediction receives zero weight.  Meanwhile, weights for predictions involving terminal nodes other than $\eta_j$ effectively receive a weight of 1, indicating no ill effect of the case deletion and providing the interpretation that influence in Bayesian tree models has a local effect in terms of prediction.
%
%The conditional independence structure of Bayesian trees allows this idea to be extended to functionals of other tree parameters, or more than single-case deletion, although the practical calculation may be come unwieldy.  
%
%%Suppose we are interested in a function of some subset of the parameters, $\theta^*.$  Suppose $\theta^*\in\check{\theta}$ and $\theta=\check{\theta}\cup \tilde{\theta}$ where $\check{\theta}\cap\tilde{\theta}=\emptyset.$  Then we can equivalently write $g(\check{\theta})$ and following the analogous factorisation as in equation (\ref{eqn:singletreepost}), the weights become
%
%%\begin{align*}
%%\frac{\pi(\theta\vert{\bf Y}_{-i})}{\pi(\theta\vert{\bf Y})} &\propto
%%\frac
%%{\prod_{k\in\eta_j:\eta_j\in\check{\theta},k\neq i}\text{N}(y_k\vert\check{\theta}))\textbf{I}[\vert\eta_j\vert-1\geq \minbot]\pi(\check{\theta})}
%%{\prod_{k\in\eta_j:\eta_j\in\check{\theta}}\text{N}(y_k\vert\check{\theta}))\pi(\check{\theta})}.
%%\end{align*}
%%
%%That is, if terminal node $\eta_j$ with case $y_i$ deleted belongs to $\check{\theta}$ we reweight as above, otherwise the weight is 1.




\subsection*{Proof of Proposition 2}

Suppose now we have a BART model involving $m$ trees.  Suppose $y_i$ lives in terminal nodes $\eta_{j1},\ldots,\eta_{jm}.$  Suppose we want to perform a (weighted) prediction at input setting $x.$  This prediction input could map exactly to each $\eta_{jl},l=1,\ldots,m$ or only a single $\eta_{jl}$ for some $l\in \lbrace 1,\ldots,m\rbrace,$ or indeed any subset of terminals between these extremes.  We will want to weight if for inputs that map to at least one of these nodes, which means $m-1$ nodes will not be in the set $\eta_{j1},\ldots,\eta_{jm}.$  Let $\boldsymbol{\eta}_a$ represent these nodes and $\boldsymbol{\eta}_b$ represent the remaining set of nodes that are not involved in predictions at $x$.  Let $\boldsymbol{\mu}_a, {\bf P}_a$ be the respective mean parameters and paths in the $m$ trees. Let $\tilde{\Theta}=\Theta\setminus \boldsymbol{\eta}_a,\boldsymbol{\mu}_a,{\bf P}_a,\sigma^2$. Finally, let ${\bf Y}_a$ and ${\bf Y}_b$ be the respective portions of the dataset.  Then,
\begin{align*}
\pi(\Theta\vert {\bf Y}) \propto f({\bf Y}_{a}\vert \boldsymbol{\mu}_a,\boldsymbol{\eta}_a,{\bf P}_a,\sigma^2)\pi(\boldsymbol{\mu}_a,\boldsymbol{\eta}_a,{\bf P}_a)\pi(\sigma^2)f({\bf Y}_b\vert \tilde{\boldsymbol{\Theta}},\boldsymbol{\mu}_a,\boldsymbol{\eta}_a,{\bf P}_a,\sigma^2)\pi(\tilde{\boldsymbol{\Theta}})\\
\propto f({\bf Y}_{a}\vert \boldsymbol{\mu}_a,\boldsymbol{\eta}_a,{\bf P}_a,\sigma^2)\pi(\boldsymbol{\mu}_a,\boldsymbol{\eta}_a,{\bf P}_a)\pi(\sigma^2)\pi(\tilde{\boldsymbol{\Theta}}\vert {\bf Y}_b,\boldsymbol{\mu}_a,\boldsymbol{\eta}_a,{\bf P}_a,\sigma^2)
\end{align*}
Integrating, we have
\begin{align*}
\int_{\tilde{\boldsymbol{\Theta}}}\pi(\Theta\vert {\bf Y})\propto \pi(\boldsymbol{\mu}_a,\boldsymbol{\eta}_a,{\bf P}_a,\sigma^2\vert {\bf Y}_a).
\end{align*}
The weights for predicting at $x$ then become
\begin{align*}
w_{(i)}^{(k)}(x) &\propto \frac{1}{f(y_i\vert \boldsymbol{\mu}_a,\boldsymbol{\eta}_a,{\bf P}_a,\sigma^2)}\prod_{l:x\in\eta_{jl}} \mathcal{I}(\vert\eta_j\vert-1\geq \minbot).
\end{align*}
Similarly, if we are interesting in predicting at $x$ such that $x$ does not involve any of the $\eta_{jl},l=1,\ldots,m$, then as in Proposition 1 the weight will be $1.$





\subsection*{Proof of Proposition 3}
Let $\mathcal{S}$ be our super-tree representation of the original BART trees $T_1,\ldots, T_m.$  Suppose $y_i$ lives in terminal node $\eta^\mathcal{S}_j$ with mean parameter $\mu^\mathcal{S}_j$ and let $P^\mathcal{S}_j$ represent the path from terminal node $j$ back to the super-tree root.  Let $\tilde{\Theta}^\mathcal{S}=\Theta^\mathcal{S}\setminus\mu^\mathcal{S}_j,P^\mathcal{S}_j,\sigma^2$ represent all other parameters making up the super-tree.  Then,
\begin{align*}
\pi(\Theta^\mathcal{S}\vert{\bf Y}) &\propto f({\bf Y}_{(j)}\vert \mu^\mathcal{S}_j,\eta^\mathcal{S}_j,P^\mathcal{S}_j,\sigma^2)\pi(\eta^\mathcal{S}_j \text{terminal})\pi(\mu^\mathcal{S}_j)\pi(P^\mathcal{S}_j)\pi(\sigma^2)f({\bf Y}_{-(j)}\vert\tilde{\Theta}^\mathcal{S},P^\mathcal{S}_j,\sigma^2)\pi(\tilde{\Theta}^\mathcal{S})\\
&\propto f({\bf Y}_{(j)}\vert \mu^\mathcal{S}_j,\eta^\mathcal{S}_j,P^\mathcal{S}_j,\sigma^2)\pi(\eta^\mathcal{S}_j  \text{terminal})\pi(\mu^\mathcal{S}_j)\pi(P^\mathcal{S}_j)\pi(\sigma^2)\pi(\tilde{\Theta}^\mathcal{S}\vert {\bf Y}_{-(j)},P^\mathcal{S}_j,\sigma^2).
\end{align*}
Integrating, we get
\begin{align*}
\int_{\tilde{\Theta}^\mathcal{S}}\pi(\Theta^\mathcal{S}\vert{\bf Y}) &\propto \pi(\mu^\mathcal{S}_j,\eta^\mathcal{S}_j,P^\mathcal{S}_j,\sigma^2\vert{\bf Y}_{(j)})
\end{align*}
and the weights for predicting at $x\in \eta^\mathcal{S}_j$ become
\begin{align*}
w_{(i)}^{(k)}(x) &\propto \frac{1}{f(y_i\vert \mu^\mathcal{S}_j,\eta^\mathcal{S}_j, P^\mathcal{S}_j,\sigma^2)}\prod_{l:x\in\eta_{kl}} \mathcal{I}(\vert\eta_{kl}\vert-1\geq \minbot).
\end{align*}
Note here that $\eta^\mathcal{S}_j=\cap_{l=1}^m\eta_{kl}$ for nodes $\eta_{kl}$ in the original BART ensemble to which $x$ maps.

Finally, as in Proposition 1, predicting at an $x$ that does not involve $\eta^\mathcal{S}_j$ has corresponding weight $1.$
